# Supplementary material for: Cloud Gaming With Foveated Graphics
Source: arXiv:1809.05823 source file (2018-09-16)
Supplement: Supplementary file 1 [file appendix.tex]

We recruited 12 participants from the Computer Science building at Aalto University. In order to make sure that their ability to play the game itself was not a confounding factor, we invited only participants that had some experience in playing First Person Shooter (FPS) games on PC (i.e. using a keyboard and mouse as the controller as opposed to using a dedicated controller). 6 participants reported having little experience, 4 participants had a medium amount of experience and 2 a high level of experience. We matched the difficulty level of the game to their self-reported skill level and their performance in the warm-up game, which was played on a medium difficulty setting for 2 minutes. We set a target of 40 kills in 5 minutes for the participant to keep the game challenging for the participants. %
The results showed that no participant was able to reach the target of 40 kills in 5 minutes, and effort and concentration remained high throughout all sessions (see Section \ref{sec:results}). This indicates that the game was challenging enough for all participants. The participants were aware only of their task, the data we collected and that the system was based on cloud gaming. Only after the experiment was finished were the participants told of the purpose of the experiment and the particular kind of foveated encoding technology that was used.

\begin{figure}
\begin{center} 
\includegraphics[width=\columnwidth]{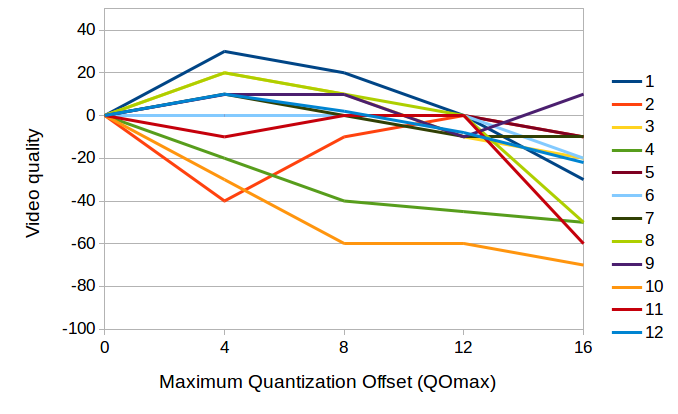} 
\caption{\small \sl Individual difference scores for the video quality per quantization level, with reference is $QO_{max} = 0$. \label{fig:video5}} 
\end{center} 
\end{figure}
\begin{figure}
\begin{center} 
\includegraphics[width=\columnwidth]{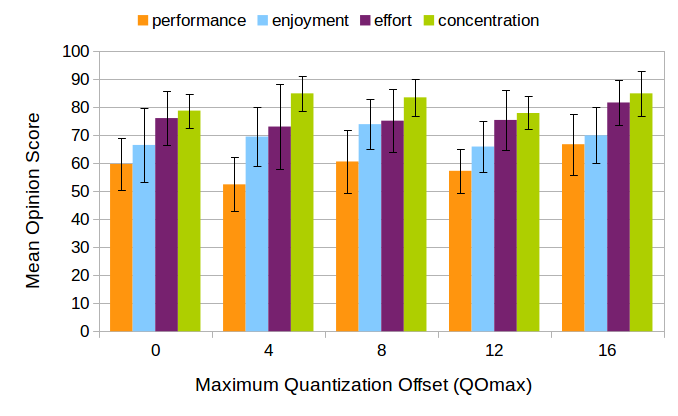} 
\caption{\small \sl Mean Opinion Scores for the task-related questions: Enjoyment, Performance satisfaction, Effort and Concentration. \label{fig:task1}} 
\end{center} 
\end{figure}
\begin{figure}
\begin{center} 
\includegraphics[width=\columnwidth]{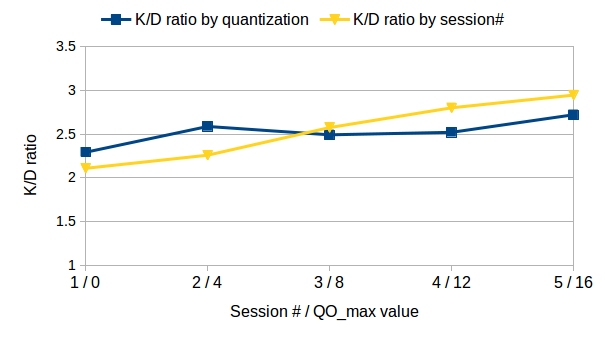} 
\caption{\small \sl The participant's mean scores plotted against the quantization level used in the session, and the session number (i.e. 1 is the first session). The score is calculated as the amount of Kills divided by the amount of Deaths: K/D ratio. \label{fig:scores}} 
\end{center} 
\end{figure}
In Figure \ref{fig:task1} we display the Mean Opinion Scores and 95\% confidence intervals for the task-related rating scales (enjoyment, performance satisfaction, effort and concentration). In Section \ref{sec:discuss} (Discussion) we further present Figures \ref{fig:video5}, \ref{fig:task1}, \ref{fig:scores} and \ref{fig:comments}, which represent the individual difference scores, MOS for task related variables, in-game scores, and participant comments, respectively.

\includegraphics[width=\columnwidth]{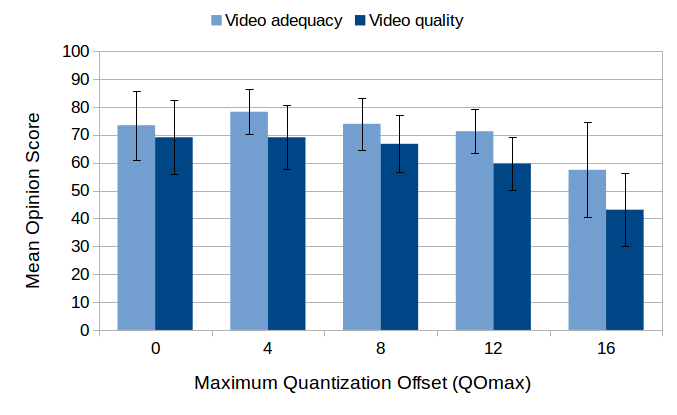} 
\caption{\small \sl Mean Opinion Scores for video quality and video adequacy, by quantization level with 95\% confidence intervals. \label{fig:video4}} 
\end{center} 
\end{figure}
